# Supplementary material for: Neutrino Event Selection in the MicroBooNE Liquid Argon Time Projection Chamber using Wire-Cell 3-D Imaging, Clustering, and Charge-Light Matching
Source: arXiv:2011.01375 source file (2021-12-26)
Supplement: Supplementary file 1 [file appendix.tex]

\section{Appendix: selected event displays from MicroBooNE data}\label{sec:appendix}
Event displays from the MicroBooNE beam-on and beam-off data are presented in this appendix.
The links to ``Bee''~\cite{wc_bee} -- a web-based 3D event display application -- are provided for each event.
In the following event displays, the red solid circles in the front view represent the measured PMT signals for the in-beam flash.
The green solid circles represent the predicted PMT signals based on the matched 3D image.
The area of the solid circle is proportional to the number of photoelectrons.

% numu candidate
\begin{figure}[htpb]  
   \centering
    \begin{overpic}[width=0.7\textwidth]{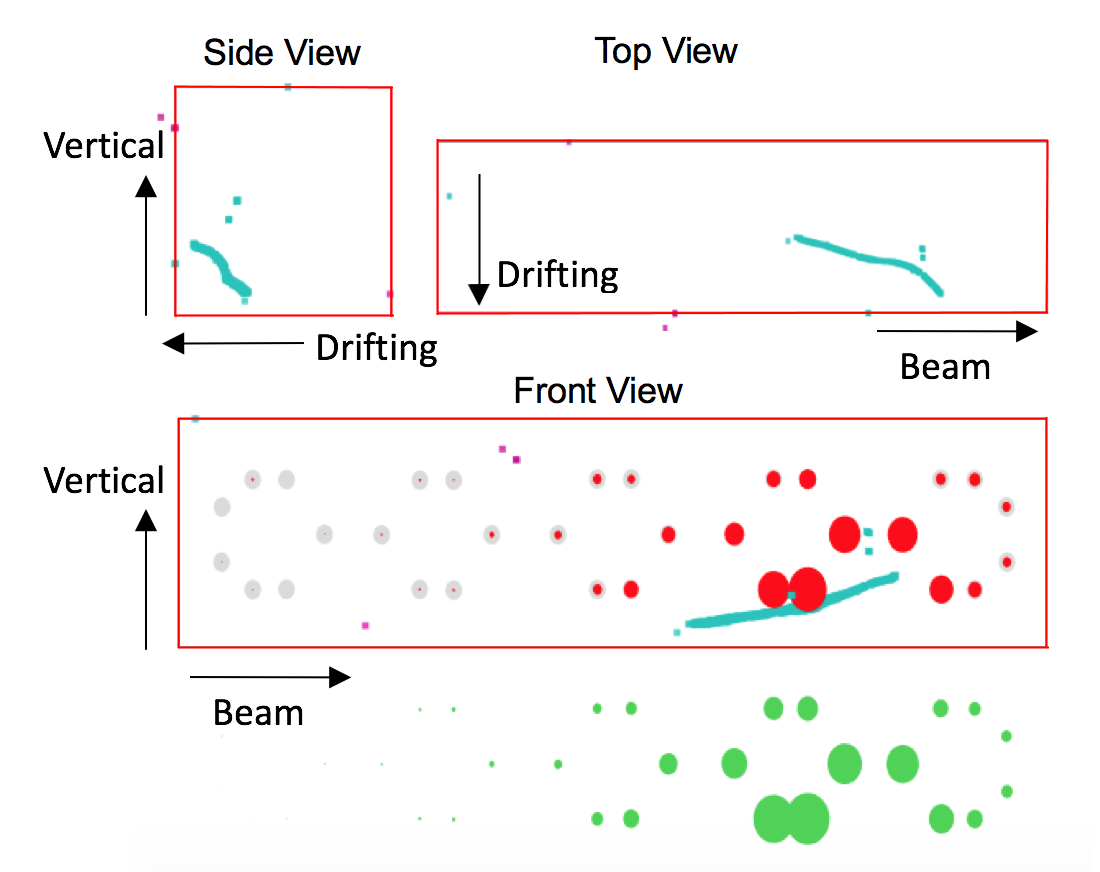}
    \put(10,78){\textbf{MicroBooNE Data}}
    \end{overpic}
   \caption{Example of a fully contained $\nu_{\mu}$ CC candidate. 
   \url{https://www.phy.bnl.gov/twister/bee/set/7ab3a69b-09cf-473e-a220-33615b6f1e55/event/12/}
    }
   \label{fig:fullnumuCC}
\end{figure}

\begin{figure}[htpb] 
   \centering
   \begin{overpic}[width=0.7\textwidth]{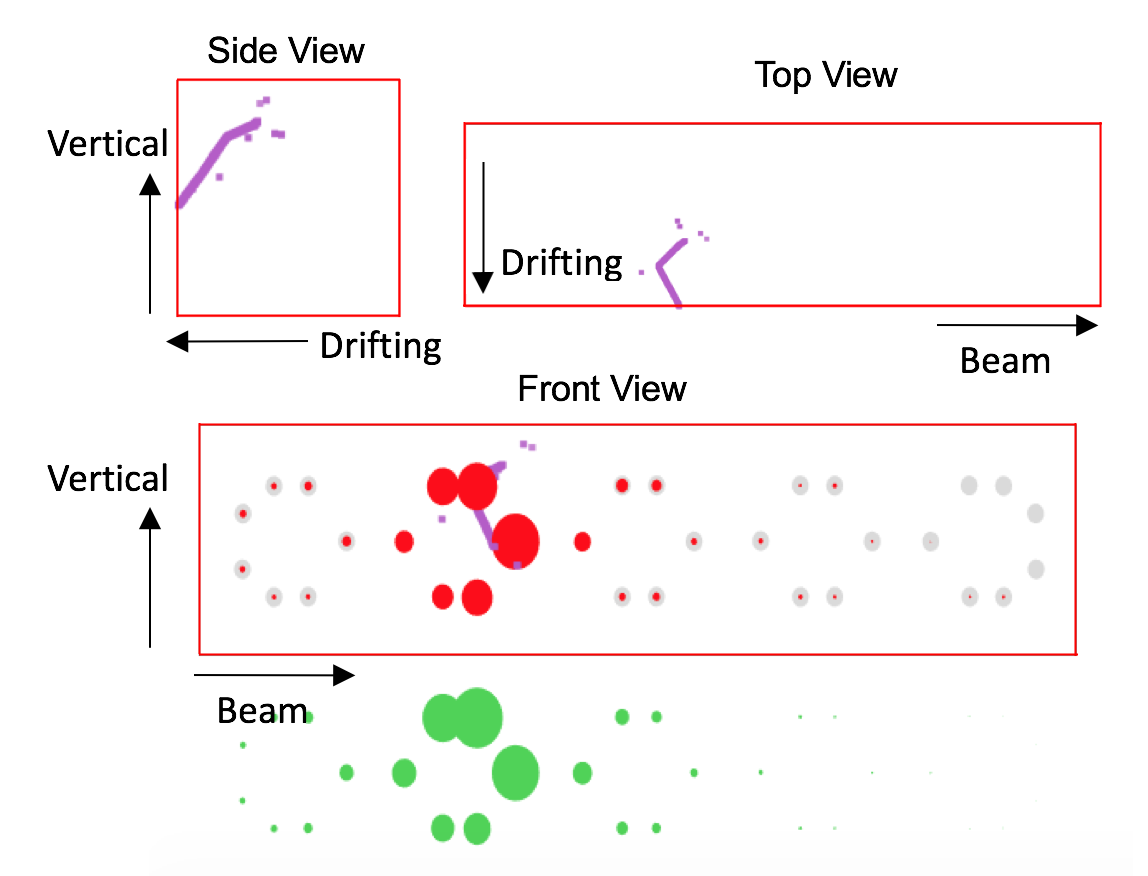}
    \put(10,75){\textbf{MicroBooNE Data}}
    \end{overpic}
   \caption{Example of a partially contained $\nu_{\mu}$ CC candidate. 
   \url{https://www.phy.bnl.gov/twister/bee/set/e06d5db6-3e16-4e05-8787-8fc3fcd3927f/event/42/}
    }
   \label{fig:partnumuCC}
 \end{figure}

%shower events
\begin{figure}[htpb]    
   \centering
   \begin{overpic}[width=1.0\textwidth]{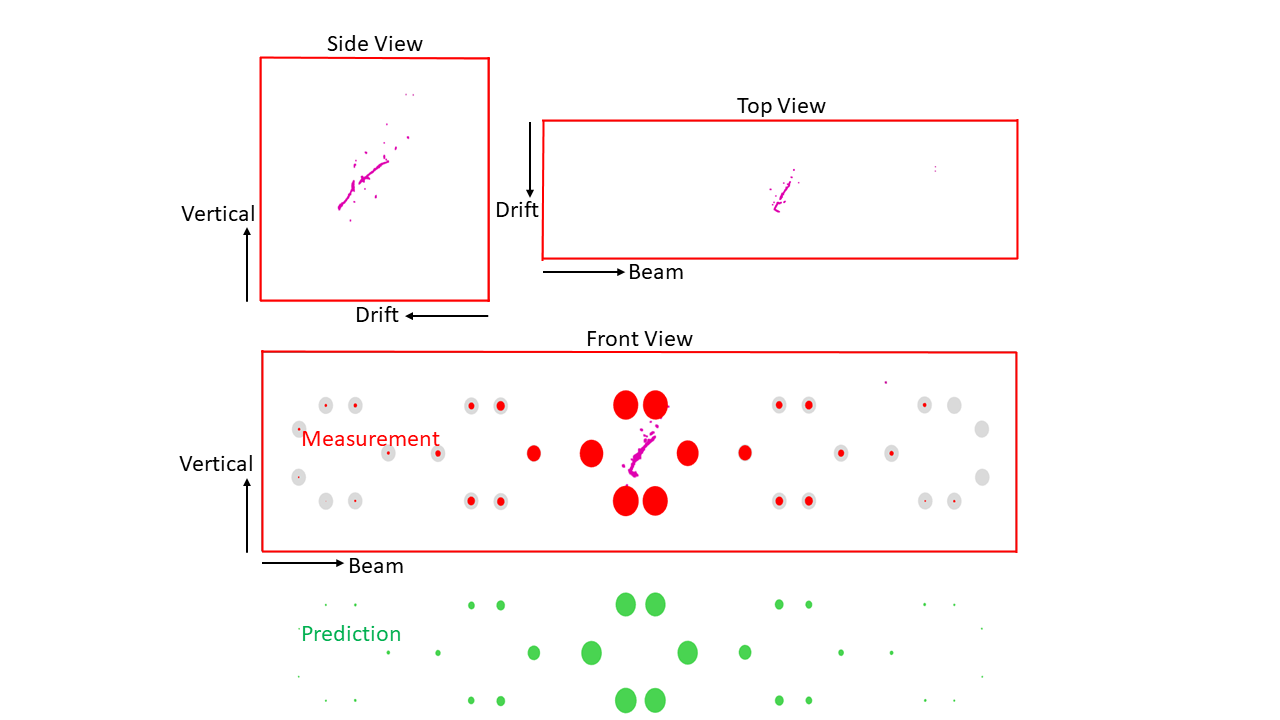}
    \put(20,55){\textbf{MicroBooNE Data}}
    \end{overpic}
   \caption{Example of a $\nu_e$ CC candidate. 
    \url{https://www.phy.bnl.gov/wire-cell/bee/set/f7bfe4cd-31b5-4eb0-9e86-7d377b1a2f82/event/196/}
    }
   \label{fig:nuE_5774}
 \end{figure}
 
 \begin{figure}[htpb]
   \centering
   \begin{overpic}[width=1.0\textwidth]{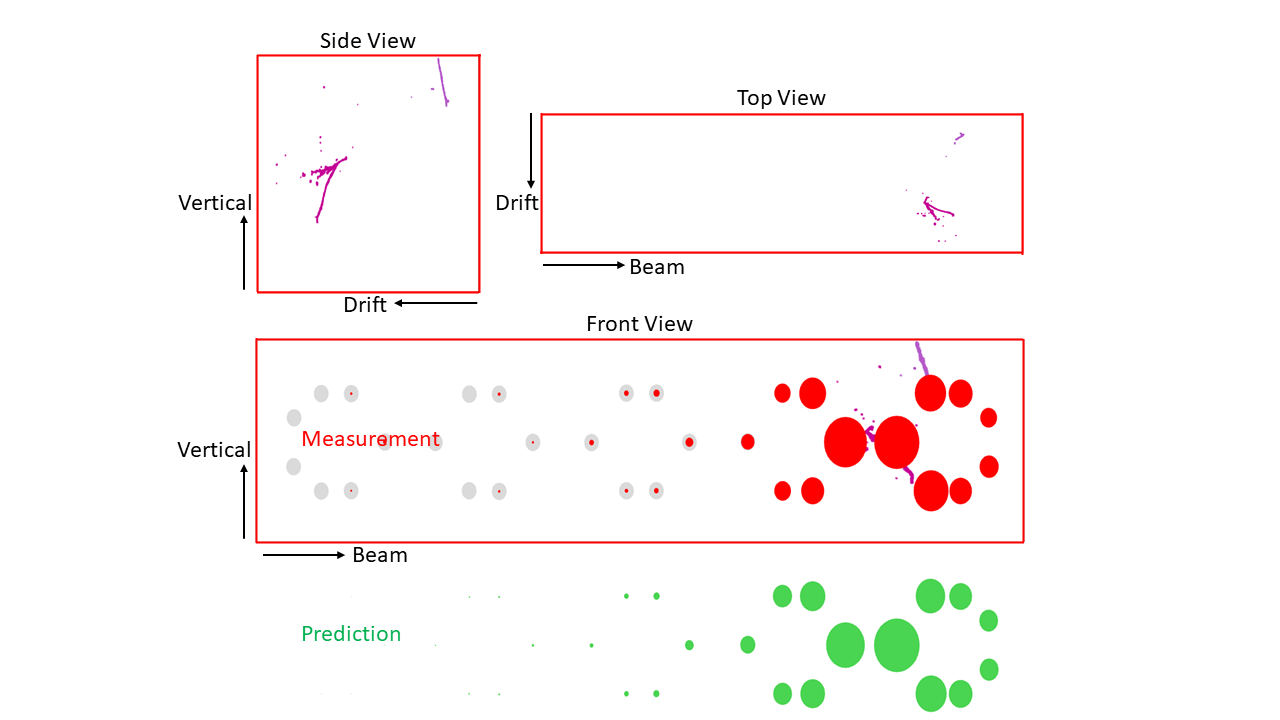}
    \put(20,55){\textbf{MicroBooNE Data}}
    \end{overpic}
   \caption{Example of a $\nu_e$ CC candidate over-clustered with a stopped muon entering from the top of the TPC active volume. 
   \url{https://www.phy.bnl.gov/wire-cell/bee/set/982c839d-e303-4aec-8e19-b9e662ec4102/event/133/}
     }
   \label{fig:nuE_5823}
 \end{figure}
 
 \begin{figure}[htpb]
   \centering
   \begin{overpic}[width=1.0\textwidth]{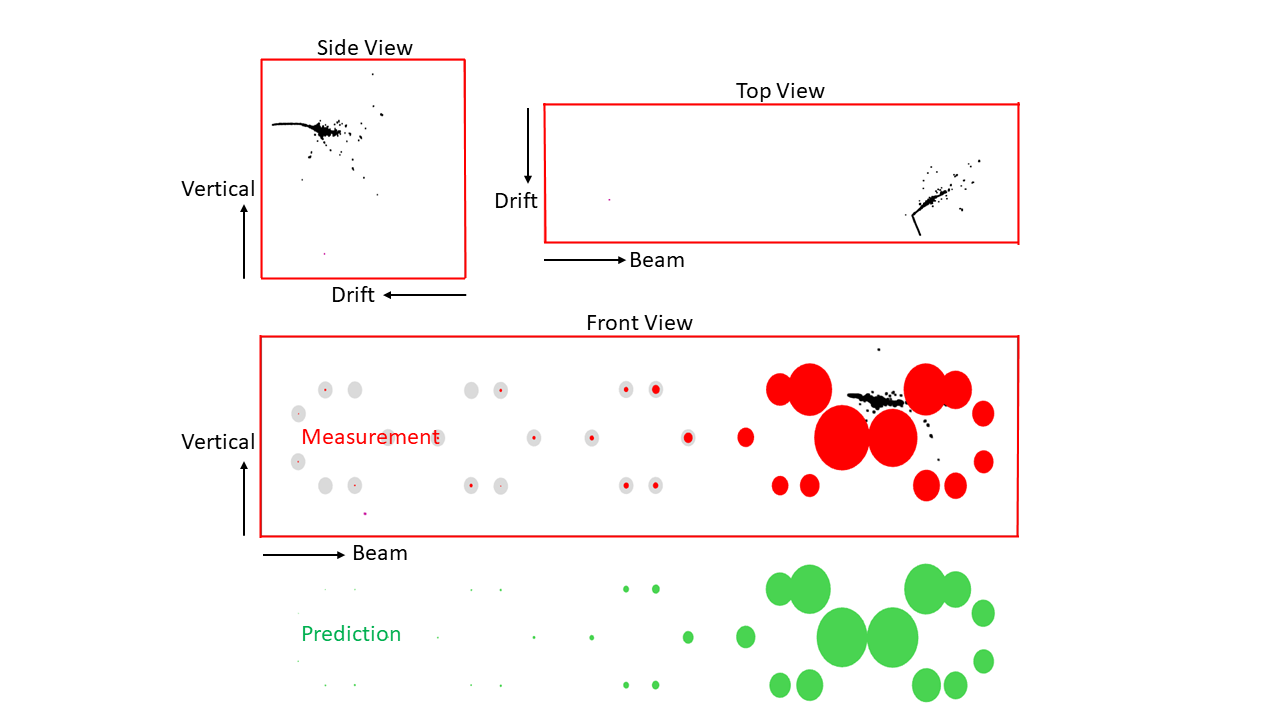}
    \put(20,55){\textbf{MicroBooNE Data}}
    \end{overpic}
   \caption{Example of a 1$e$1$p$ $\nu_e$ CC candidate. 
   \url{https://www.phy.bnl.gov/wire-cell/bee/set/8ce87fc2-ecd0-49c2-b227-2deec9a6a566/event/122/}
     }
   \label{fig:nuE_5906}
 \end{figure}

 \begin{figure}[htpb]
   \centering
   \begin{overpic}[width=1.0\textwidth]{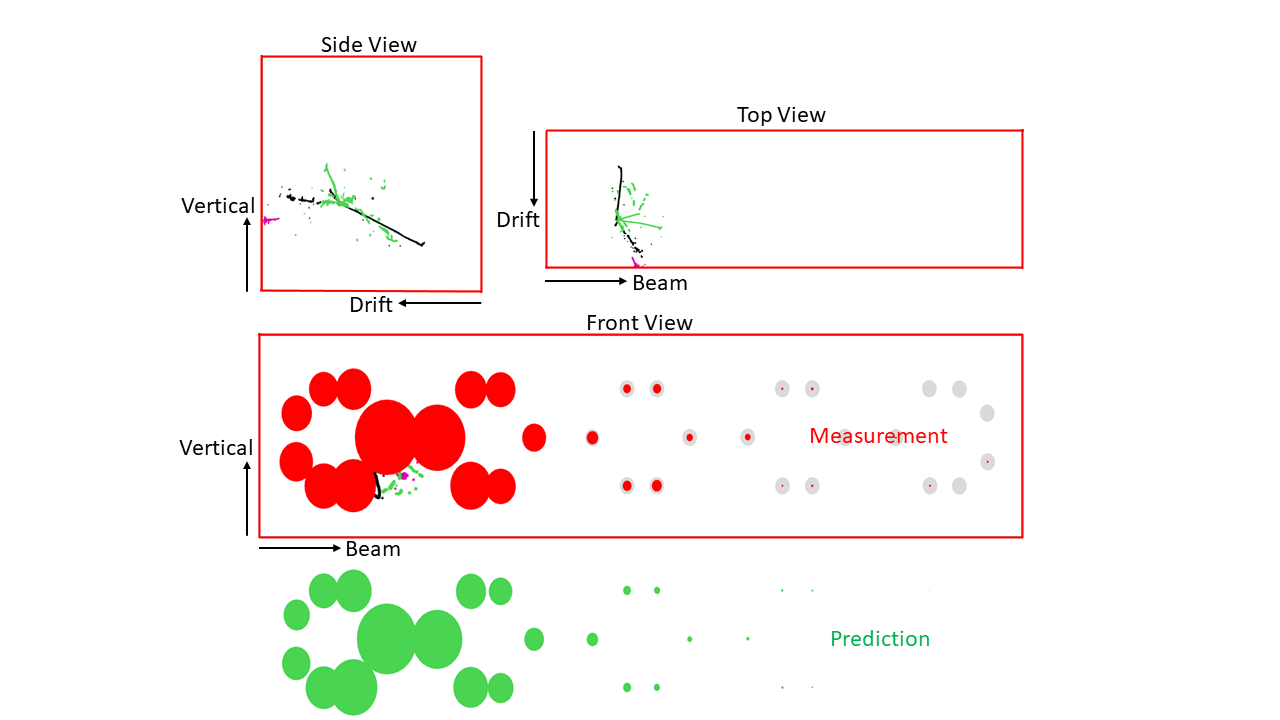}
    \put(20,55){\textbf{MicroBooNE Data}}
    \end{overpic}
   \caption{Example of an event that probably contains more than one $\pi^{0}$ event. 
   \url{https://www.phy.bnl.gov/wire-cell/bee/set/8ce87fc2-ecd0-49c2-b227-2deec9a6a566/event/58/}
     }
   \label{fig:pi0_5896}
 \end{figure}

\begin{figure}[htpb]
   \centering
   \begin{overpic}[width=1.0\textwidth]{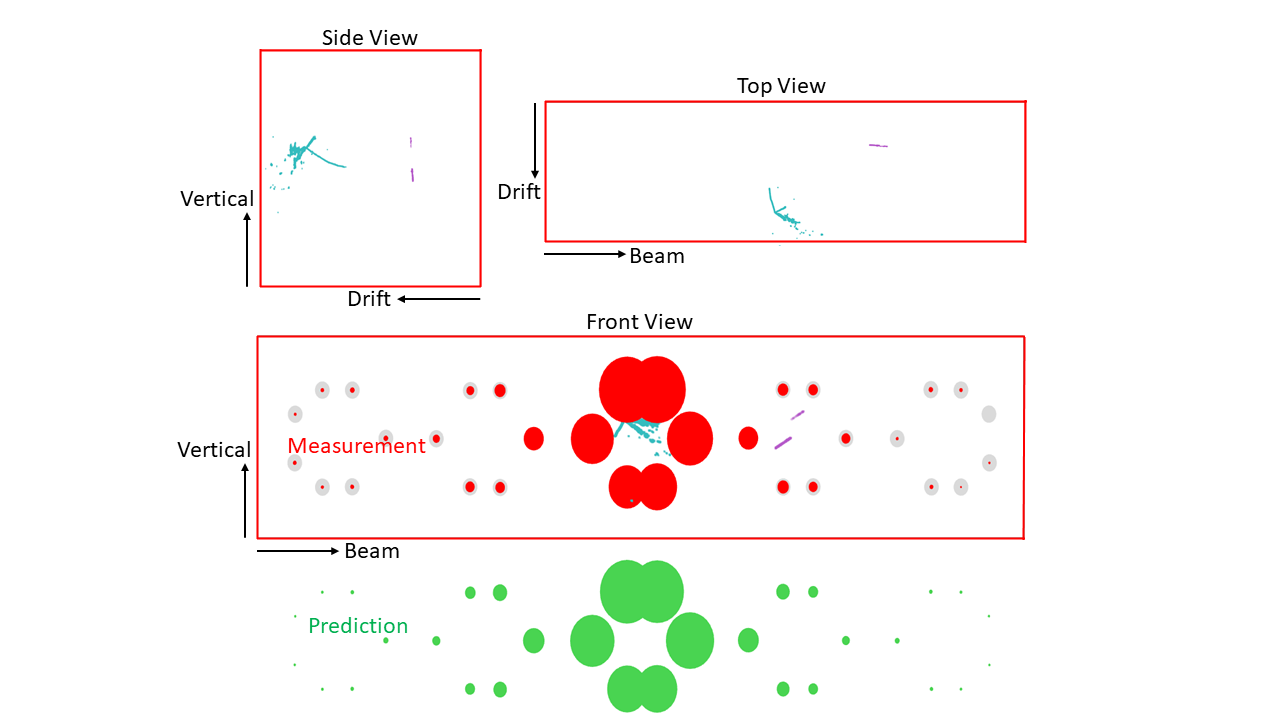}
    \put(20,55){\textbf{MicroBooNE Data}}
    \end{overpic}
	\caption{Example of an event with a possibility of two EM showers ($e^{+}e^{-}$?)  connected to the primary vertex
	    %Example of two EM showers ($e^{+}e^{-}$?) connected to the primary vertex. 
   \url{https://www.phy.bnl.gov/wire-cell/bee/set/8122be11-3423-4b7e-95fd-08c6e9791079/event/194/}
    }
   \label{fig:e+e-_5179}
 \end{figure}

% through-going muon
\begin{figure}[htpb]
   \centering
   \begin{overpic}[width=0.7\textwidth]{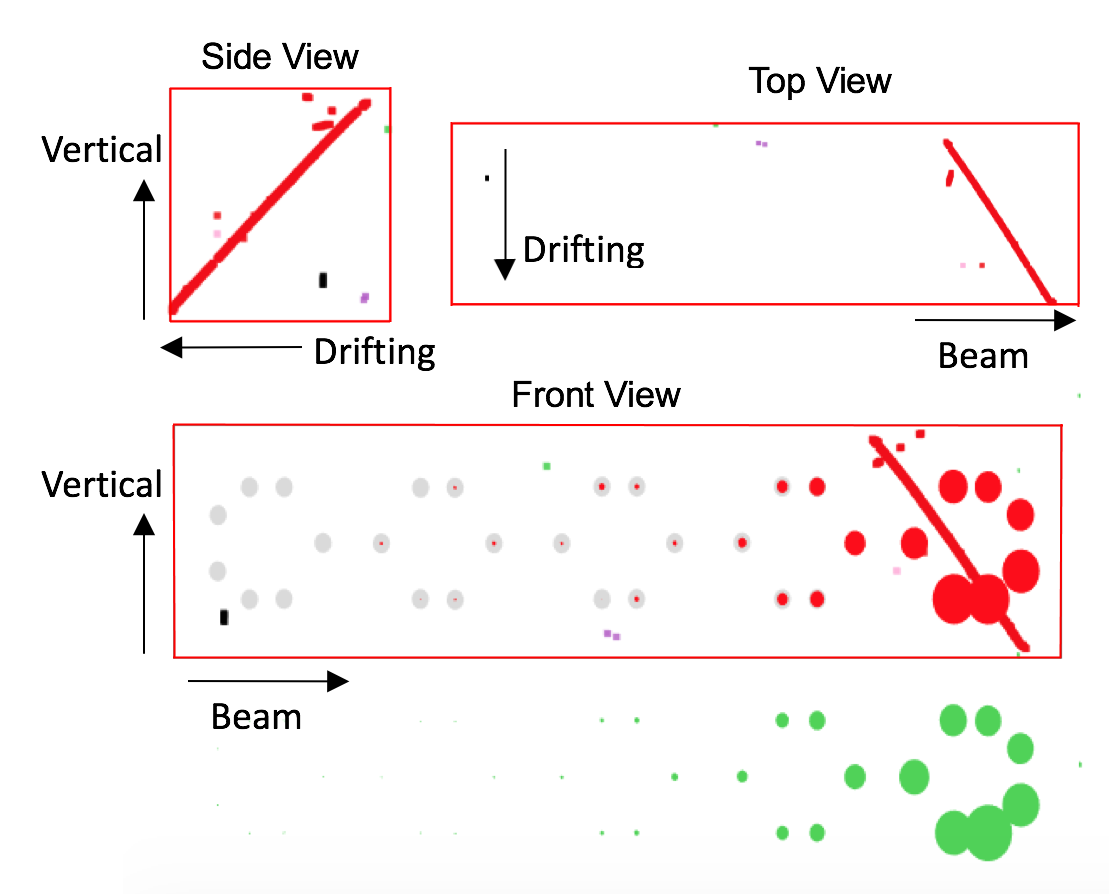}
    \put(10,80){\textbf{MicroBooNE Data}}
    \end{overpic}
   \caption{Example of a through-going muon from beam-off data. The upper end in the side view is on the space charge boundary. 
   \url{https://www.phy.bnl.gov/twister/bee/set/7ab3a69b-09cf-473e-a220-33615b6f1e55/event/67/}
    }
   \label{fig:throughmuon}
\end{figure}

% stopped muon with a Michele electron
 \begin{figure}[htpb] 
   \centering
   \begin{overpic}[width=0.7\textwidth]{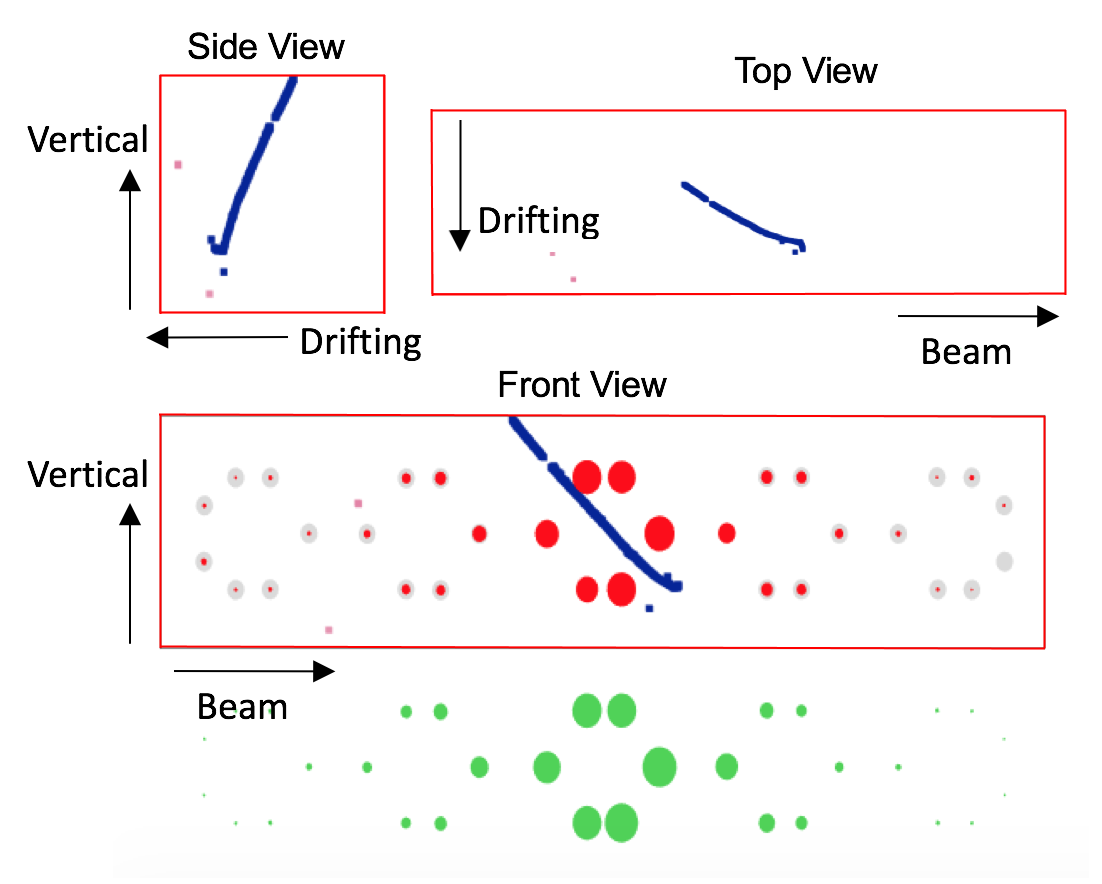}
    \put(10,80){\textbf{MicroBooNE Data}}
    \end{overpic}
   \caption{Example of a stopped muon with a Michel electron from beam-off data. 
   \url{https://www.phy.bnl.gov/twister/bee/set/7ab3a69b-09cf-473e-a220-33615b6f1e55/event/83/}
     }
   \label{fig:stoppedmuonMichel}
 \end{figure}

% useful bee display
% NC https://www.phy.bnl.gov/twister/bee/set/ae1aaadb-2380-4ab6-b396-df4760b2a502/event/list/ 
% numuCC https://www.phy.bnl.gov/twister/bee/set/133ded40-d934-47d5-940c-fb747731ea20/event/list/
% numuCC https://www.phy.bnl.gov/twister/bee/set/248afd9e-1a6d-4216-af6a-c5f602fea514/event/list/
% nueCC https://www.phy.bnl.gov/twister/bee/set/999cb1a5-68b6-4e60-a7c7-1d3143ab8db8/event/list/ 
